# Supplementary material for: How Adults Understand What Young Children Say
Source: arXiv:2206.07807 source file (2023-03-16)
Supplement: Supplementary file 1 [file supplement.tex]

%For communicative successes, we evaluate the probability that each model assigns to the `correct' gloss.\footnote{`Correct' with respect to the adult listener's guess. We have not data as to whether this was the word intended by the child speaker.} 
%Taking the average surprisal (negative log probability\footnote{For statistics-oriented readers, this is the per-instance log-likelihood of the data under the model.}) assigned to `correct' words in the context of communicative successes offers a way to evaluate which models best predict the words recovered by adults, and therefore to quantify the contribution of priors to successful recovery of a conventional word in the adult language.

%For communicative successes, we evaluate the probability that each model assigns to the `correct' gloss.\footnote{`Correct' with respect to the adult listener's guess. We have not data as to whether this was the word intended by the child speaker.} 
%Taking the average surprisal (negative log probability\footnote{For statistics-oriented readers, this is the per-instance log-likelihood of the data under the model.}) assigned to `correct' words in the context of communicative successes offers a way to evaluate which models best predict the words recovered by adults, and therefore to quantify the contribution of priors to successful recovery of a conventional word in the adult language.

\footnote{Diphthongs were treated as two phones for edit distance calculations.}

 (among words on the CDI, \citealp{fenson2007macarthur}, 98\% meet this criterion)
 
 The limitation to single syllable segments in both cases reflects difficulties in computing prior probabilities for multi-word sequences (see Priors, below).  
Without such a filter, transcribed material for a single \texttt{yyy} token could contain multiple words. e.g. /ju v\textipa{@} ma\textipa{I} t\textipa{A} [g\textipa{@}t\textipa{I}u]/ (with [g\textipa{@}t\textipa{I}u] glossed as \texttt{yyy} most likely \textit{get you}.)
%eb: this isn't rendering right
%We return in the Discussion to approaches (e.g. multi-word infilling) that would cover such cases.
The exclusion of words with recording failures or additional communicative failures was motivated by modeling limitations on conditioning on contexts that include these tokens. %eb  say that simpler and earlier

\noindent \textbf{Phonetic Pre-processing} IPA citation forms for word candidates were retrieved from the CMU dictionary, taking the first pronunciation in  cases with multiple pronunciations. 
We use citation forms from CMU to provide broader coverage over words than that available in PhonBank.
To reconcile distinctions between narrow transcription in the Providence corpus and broad transcription in the CMU dictionary, markers for aspiration and nasalization were removed from Providence transcriptions, and some non-point vowels and forms of `r' were collapsed to maximize coverage of citation forms in Phonbank. 
83\% of adjusted Providence tokens were in the adjusted CMU inventory \todo{check again; I fixed more stuff}).
